# Supplementary material for: Topological Symmetry Enhanced Graph Convolution for Skeleton-Based Action Recognition
Source: arXiv:2411.12560 source file (2024-11-20)
Supplement: Supplementary file 1 [file X_suppl.tex]

\clearpage
\setcounter{page}{1}
\setcounter{section}{0}

\maketitlesupplementary

In the supplementary material, we present details about the architecture setup as well as extended experiments and analysis, including additional performance evaluations on certain action classes and visualizations to illustrate the effects of our modules. 
\section{Detailed Architecture}
\label{sec:architecture-supp}
\begin{table}[h]
\centering
\caption{Detailed architecture of TSE-GCN. $T$ refers to the number of frames. First two hyperparameters are the input and output channel. The third hyperparameter for TC is the stride.}
\label{tab:supp-arch}
\resizebox{0.4\textwidth}{!}{
\begin{tabular}{l|cc}
\hline
Layers & Output Temporal Size & Hyperparameters \\
\hline
Embed & $T$ & PE: 3 $C$ \\
\hline
Block 1-3 & $T$ & \makecell{GC: $C$ $C$ \\ TC: $C$ $C$ 1} \\
\hline
Block 4 & $\frac{T}{2}$ & \makecell{GC: $C$ 2$C$ \\ TC: 2$C$ 2$C$ 2} \\
\hline
Block 5-6 & $\frac{T}{2}$ & \makecell{GC: 2$C$ 2$C$ \\ TC: 2$C$ 2$C$ 1} \\
\hline
Block 7 & $\frac{T}{4}$ & \makecell{GC: 2$C$ 4$C$ \\ TC: 4$C$ 4$C$ 2} \\
\hline
Block 8-9 & $\frac{T}{4}$ & \makecell{GC: 4$C$ 4$C$ \\ TC: 4$C$ 4$C$ 1} \\
\hline
Classifier & 1 & - \\
\hline
\end{tabular}
}
\end{table}

The detailed architecture of TSE-GCN is shown in table \ref{tab:supp-arch}. $T$ is 64 for NTU RGB+D 60\cite{shahroudy2016ntu} and NTU RGB+D 120\cite{liu2019ntu}. For NW-UCLA\cite{wang2014cross}, $T$ is 52. $C$ is the basic channel which is set as 64 for TSE-GCN. At the Block 4 and 7, the strides of MBDTC are set to 2 to reduce the temporal dimension by half. PE denotes the learnable absolute positional embedding from \cite{chi2022infogcn}.

\section{Extended Experiments and Analysis}
\label{sec:analysis}

\subsection{Performance Analysis on Action Classes}
In the paper, we utilize GPT4\cite{achiam2023gpt} to identify topological symmetry related classes within NTU RGB+D 120\cite{liu2019ntu}, which are shown in table \ref{tab:related}. Here we present the accuracy difference of all classes between TSE-GC and two representative GCs, namely ST-GC\cite{yan2018spatial} and CTR-GC\cite{chen2021channel}, in Fig.\ref{fig:baseline_overall} and Fig.\ref{fig:ctr_overall}. Our MBDTC is adopted as the temporal modeling module for a fair comparison between GCs. We observe improved accuracies on additional action classes related to the cooperation of symmetric joints, which are not identified by GPT4, such as \enquote{apply cream on hand back}, \enquote{take off head phone} and \enquote{tear up paper}. We further analyze the classes where our TSE-GC exhibits reduced performance and identify three potential reasons: 

\noindent (1) The actions do not involve the cooperation of symmetric joints. In this case, the reactivation mechanism of TSE-GC slightly damages the performance by unnecessarily reactivating symmetric interactions. 

\noindent (2) The actions involves topological symmetric motions which are not effectively captured by the KNN algorithm. For example, in the case of \enquote{arm circles}, the correlation between circled arms is not reactivated because they are spatially distant from each other and thus not captured. 

\noindent (3) The actions exhibit a reversed temporal order compared to some other classes and are misclassified, such as \enquote{wear jacket} and \enquote{take off a jacket}. 

Despite the limitations, we observe our TSE-GC demonstrates significant accuracy improvements on hard action classes, provided in table \ref{tab:HARD}. These actions typically involve subtle interactions between fingers or toes and fine-grained movements that are difficult to capture using only skeleton data. On average, Our TSE-GC exceeds ST-GC and CTR-GC by 6.25\% and 5.35\% on these classes respectively, demonstrating the ability to capture subtle interactions.     

\begin{table}[t]
\centering
\caption{Comparison of performance between GCs on hard classes.}
\label{tab:HARD}
\resizebox{0.4\textwidth}{!}{
\begin{tabular}{c|ccc}
\hline
\multirow{2}{*}{Action} & \multicolumn{3}{c}{Accuracies(\%)} \\ 
\cline{2-4}
                        & ST-GC   & CTR-GC   & TSE-GC \\
\hline
staple book& 36.8 & 28.9 & 37.7 \\
open bottle& 72.4 & 73.5 & 80.3 \\
counting money& 52.6 & 57.0 & 58.1 \\
cutting nails& 60.1 & 67.1 & 68.5 \\
play magic cube & 69.9 & 73.6 & 77.8 \\
typing on a keyboard & 69.1 & 66.2 & 76.0 \\
\hline
\end{tabular}
}
\end{table}

\begin{table}[t]
\centering
\caption{Topological symmetry related classes within NTU RGB+D 120 identified by GPT4\cite{achiam2023gpt}.}
\label{tab:related}
\resizebox{0.47\textwidth}{!}{
\begin{tabular}{cc|cc}
\hline
Label & Action & Label & Action\\
\hline
3&brushing teeth & 4&brushing hair\\
10&clapping & 26&hopping\\
27&jump up & 34&rub two hands together\\
35&nod head/bow & 39&put the palms together\\
40&cross hands in front & 49&use a fan/feeling warm\\
50&punching/slapping other person & 57&touch other person's pocket\\
58&handshaking & 63&shoot at the basket\\
80&squat down & 93&shake fist\\
95&hands up & 96&cross arms\\
97&arm circles & 99&running on the spot\\
100&butt kicks & 101&cross toe touch\\
102&side kick & 104&stretch oneself\\
106&hit other person with something &112&high-five\\
120&finger-guessing game\\

\hline
\end{tabular}
}
\end{table}
 
\begin{figure*}[htbp]
	\centering
	%\fbox{\rule{0pt}{2in} \rule{0.9\linewidth}{0pt}}
	\includegraphics[width=0.83\linewidth]{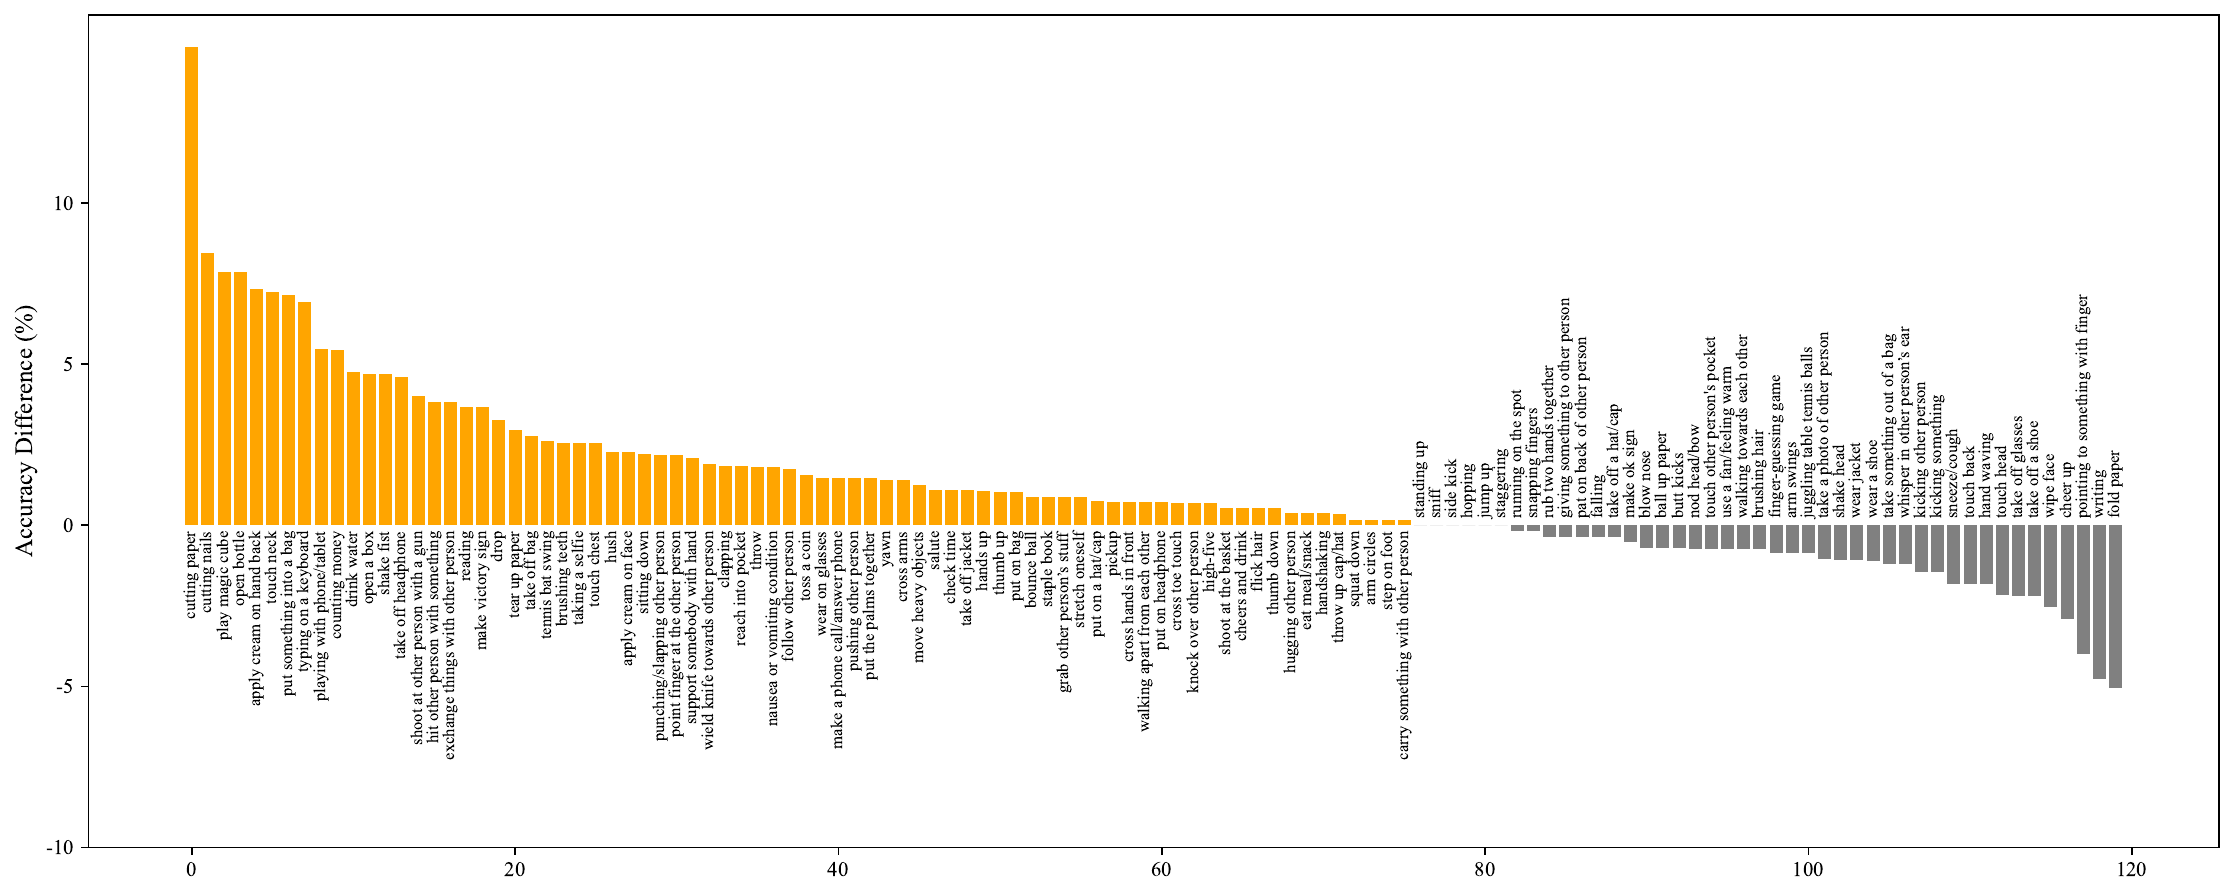}
	
	\caption{Accuracy difference(\%) between TSE-GC and ST-GC.}
	\label{fig:baseline_overall}
\end{figure*}

 \begin{figure*}[htbp]
	\centering
	%\fbox{\rule{0pt}{2in} \rule{0.9\linewidth}{0pt}}
	\includegraphics[width=0.83\linewidth]{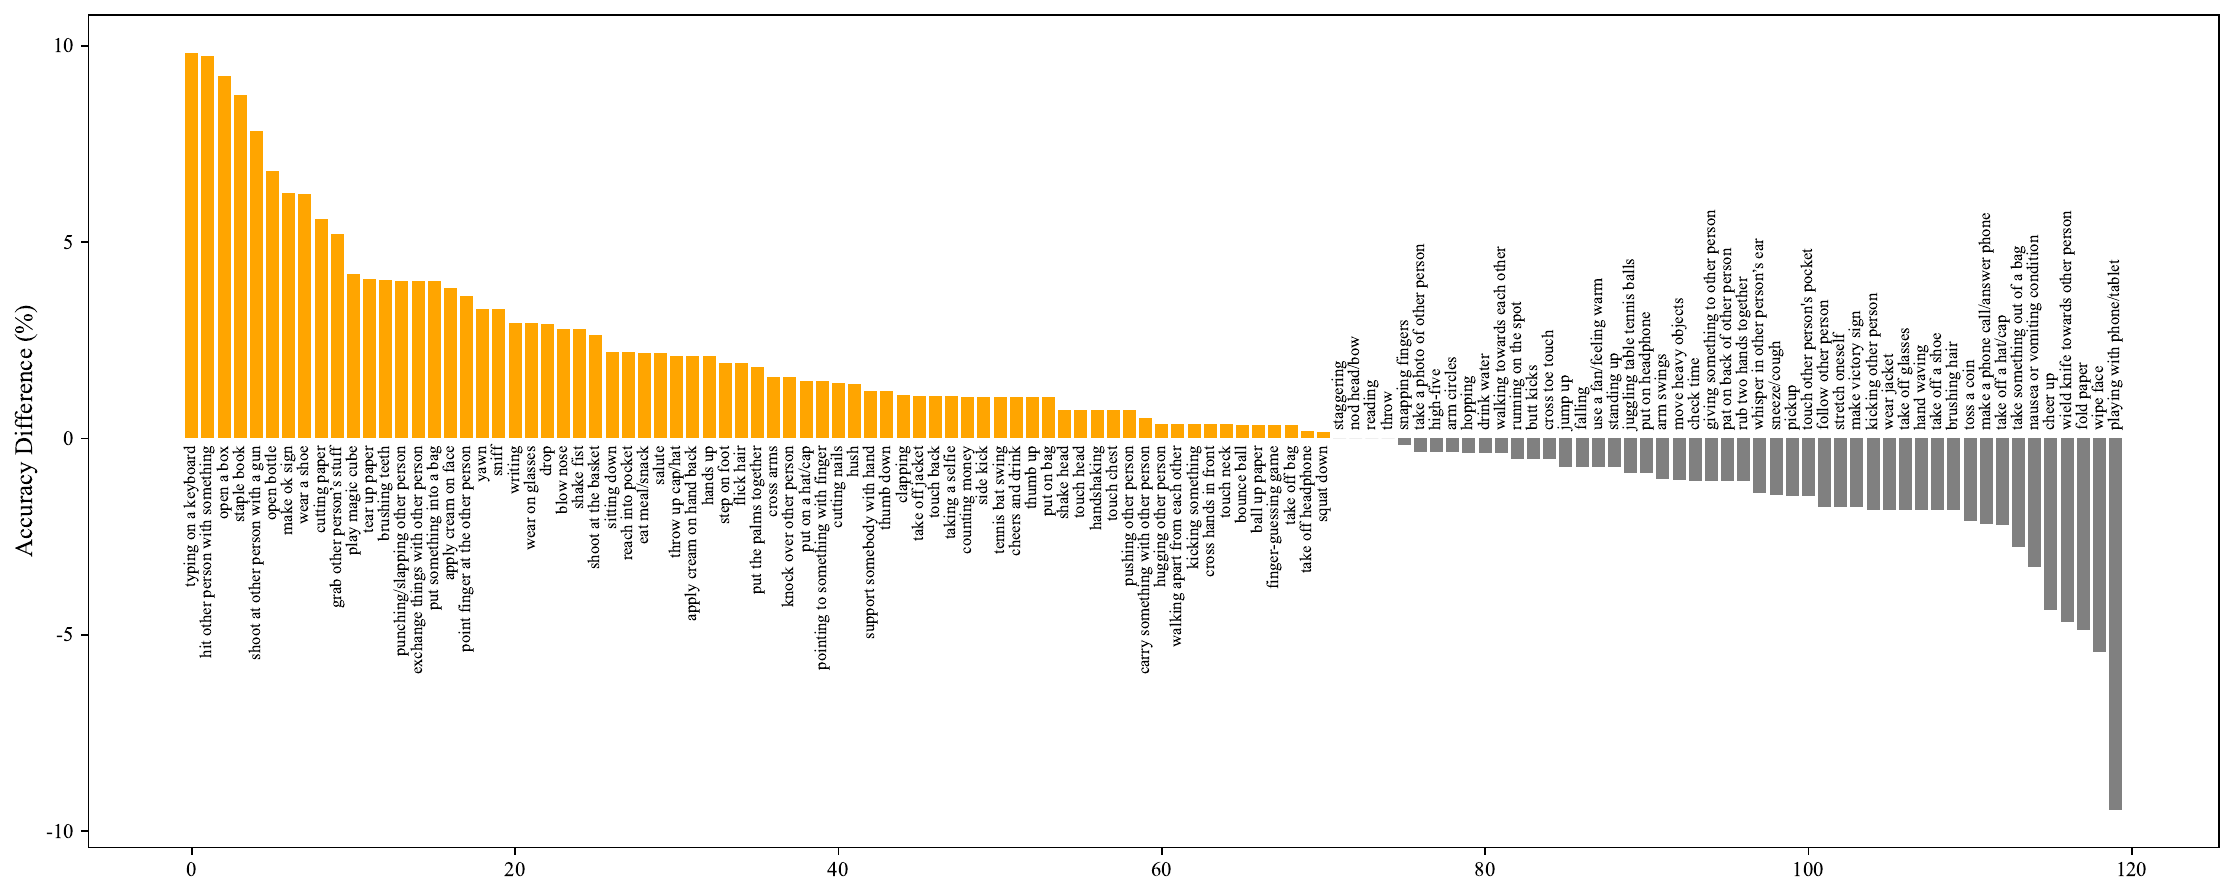}
	
	\caption{Accuracy difference(\%) between TSE-GC and CTR-GC.}
	\label{fig:ctr_overall}
\end{figure*}

\subsection{Visualization of Learned Topologies}

To verify the effectiveness of incorporating both flexibility and physical constraints rooted in topological symmetry, we provide the learned topologies of our TSE-GC in Fig.\ref{fig:As}. They are not decoupled as it is meaningless to consider all elements in $\mathbf{A_s}$ due to our reactivation mechanism. The visualizations reveal the capacity of TSE-GC to balance the flexibility and topological symmetry adaptively and correspond to our initial design. 

\begin{figure*}
    \centering
    \begin{subfigure}[b]{0.15\textwidth}
        \centering
        \includegraphics[width=1.0\linewidth]{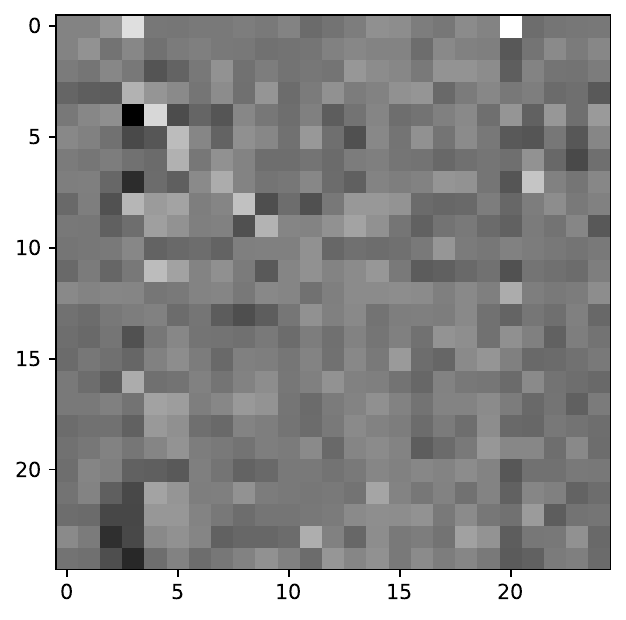}
        \caption{Layer 1.}
    \end{subfigure}
    \hfill
    \begin{subfigure}[b]{0.15\textwidth}
        \centering
        \includegraphics[width=1.0\linewidth]{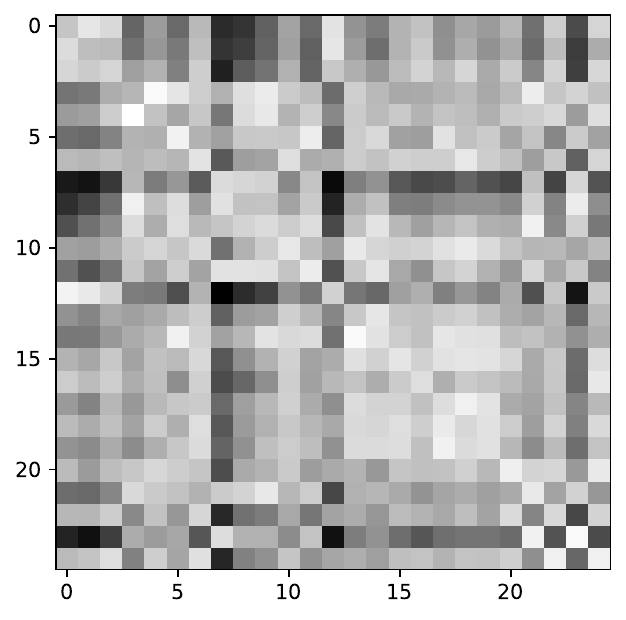}
        \caption{Layer 2.}
    \end{subfigure}
    \hfill
    \begin{subfigure}[b]{0.15\textwidth}
        \centering
        \includegraphics[width=1.0\linewidth]{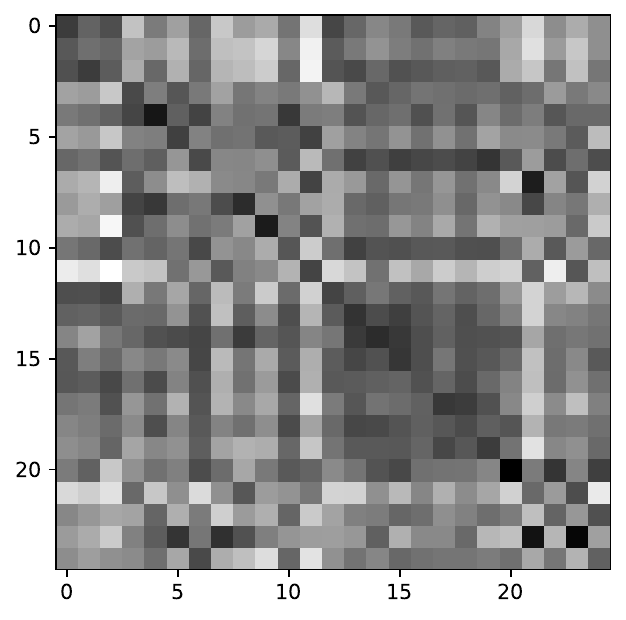}
        \caption{Layer 3.}
    \end{subfigure}
    \hfill
    \begin{subfigure}[b]{0.15\textwidth}
        \centering
        \includegraphics[width=1.0\linewidth]{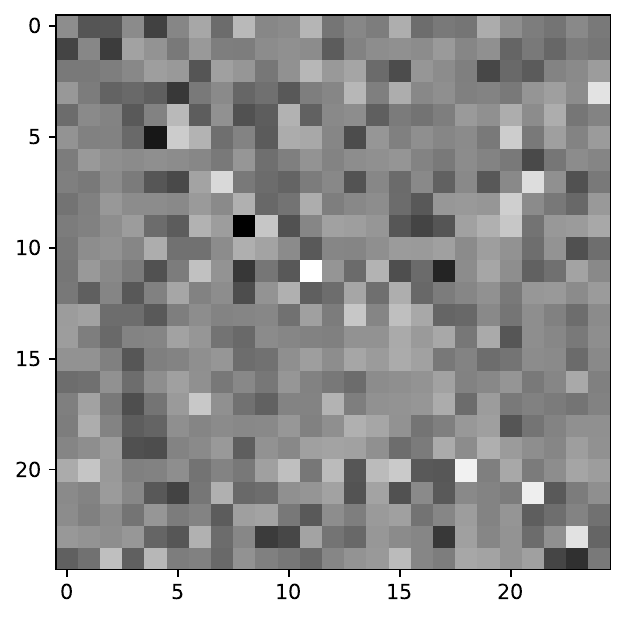}
        \caption{Layer 4.}
    \end{subfigure}
    \hfill
    \begin{subfigure}[b]{0.15\textwidth}
        \centering
        \includegraphics[width=1.0\linewidth]{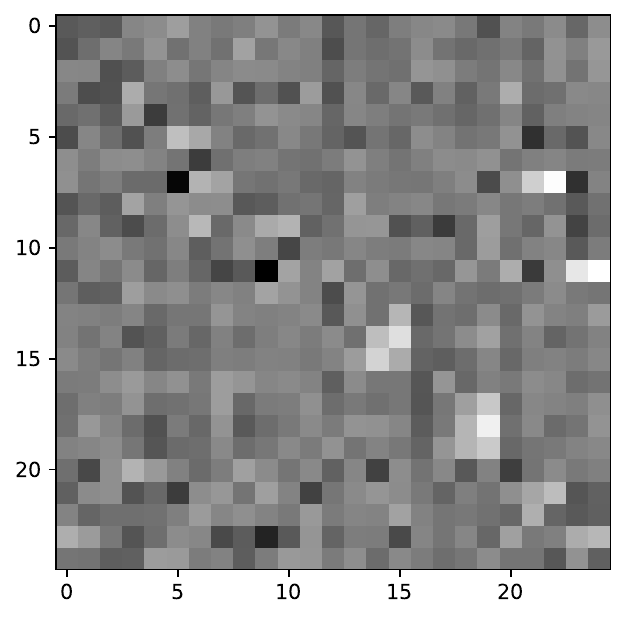}
        \caption{Layer 5.}
    \end{subfigure}

    \begin{subfigure}[b]{0.15\textwidth}
        \centering
        \includegraphics[width=1.0\linewidth]{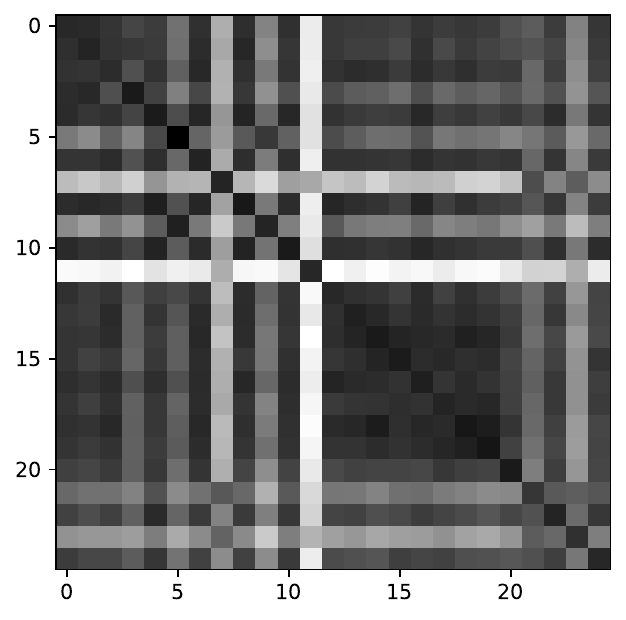}
        \caption{Layer 6.}
    \end{subfigure}
    \hfill
    \begin{subfigure}[b]{0.15\textwidth}
        \centering
        \includegraphics[width=1.0\linewidth]{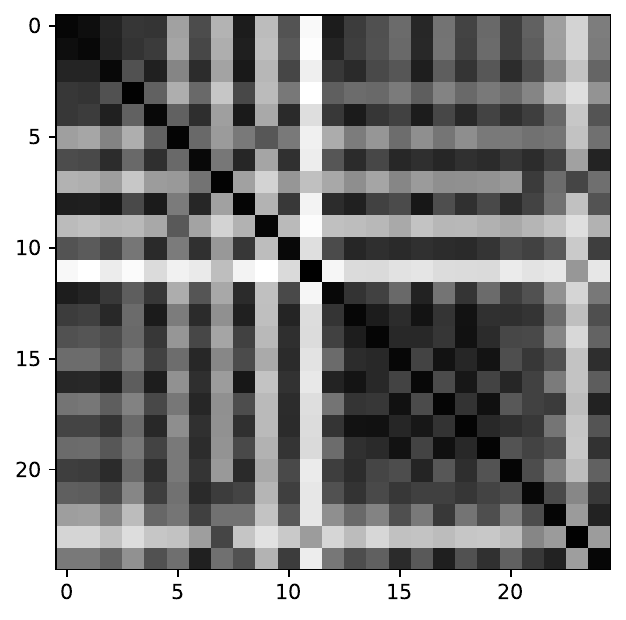}
        \caption{Layer 7.}
    \end{subfigure}
    \hfill
    \begin{subfigure}[b]{0.15\textwidth}
        \centering
        \includegraphics[width=1.0\linewidth]{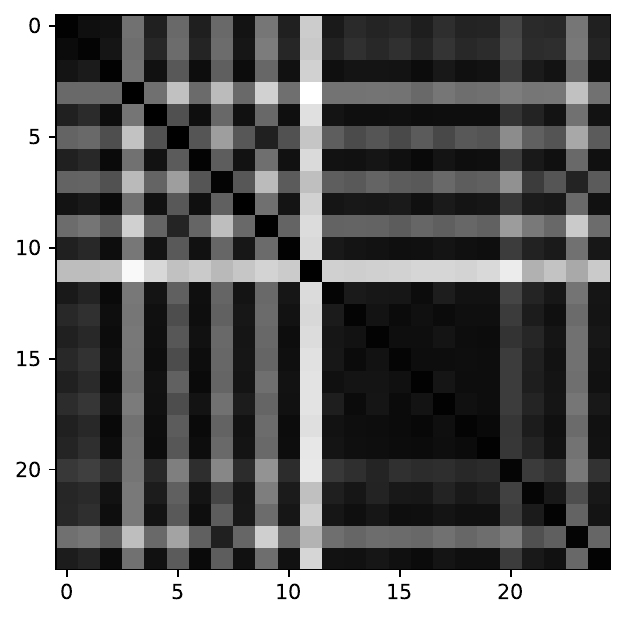}
        \caption{Layer 8.}
    \end{subfigure}
    \hfill
    \begin{subfigure}[b]{0.15\textwidth}
        \centering
        \includegraphics[width=1.0\linewidth]{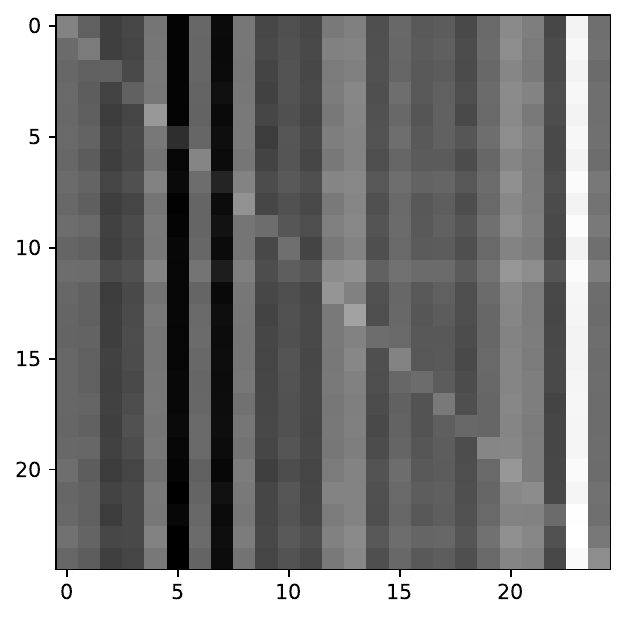}
        \caption{Layer 9.}
    \end{subfigure}
    \caption{The learned topologies of our TSE-GCN. Darker colors stand for larger weights. It can be seen that TSE-GC layers adaptively balance the flexibility and topological symmetry based on different levels of semantics. }
    \label{fig:As}
\end{figure*}

\subsection{Visualization of Temporal Offsets}

We provide the averaged sampling locations of MBDTC in Fig.\ref{fig:supp-DTC}. The original sampling offsets are -2,-1,0,1,2 (dilation is 1) and -4,-2,0,2,4 (dilation is 2). It can be seen that as we move towards the upper layers, the sampling offsets exhibit significant variations, demonstrating the advantage of MBDTC by dynamically adjusting receptive fields. An interesting finding is that positive offsets seem to fluctuate greater than negative ones. 

 \begin{figure}[H]
	\centering
	%\fbox{\rule{0pt}{2in} \rule{0.9\linewidth}{0pt}}
	\includegraphics[width=\linewidth]{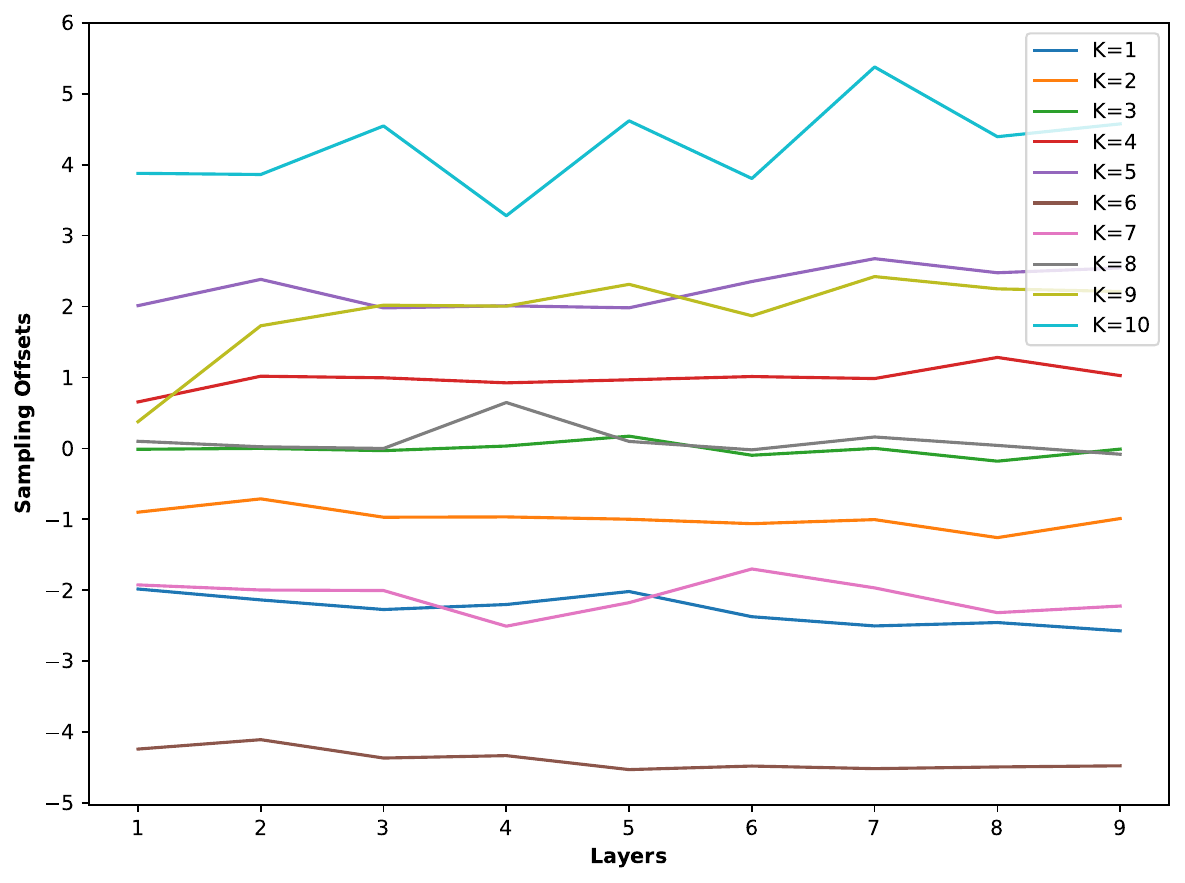}
	
	\caption{The deformable sampling offsets of our MBDTC module. The offsets across temporal frames are averaged as the temporal size varies between layers.}
	\label{fig:supp-DTC}
\end{figure}

% % 
% Having the supplementary compiled together with the main paper means that:
% % 
% \begin{itemize}
% \item The supplementary can back-reference sections of the main paper, for example, we can refer to \cref{sec:intro};
% \item The main paper can forward reference sub-sections within the supplementary explicitly (e.g. referring to a particular experiment); 
% \item When submitted to arXiv, the supplementary will already included at the end of the paper.
% \end{itemize}
% % 
% To split the supplementary pages from the main paper, you can use \href{https://support.apple.com/en-ca/guide/preview/prvw11793/mac#:~:text=Delete%20a%20page%20from%20a,or%20choose%20Edit%20%3E%20Delete).}{Preview (on macOS)}, \href{https://www.adobe.com/acrobat/how-to/delete-pages-from-pdf.html#:~:text=Choose%20%E2%80%9CTools%E2%80%9D%20%3E%20%E2%80%9COrganize,or%20pages%20from%20the%20file.}{Adobe Acrobat} (on all OSs), as well as \href{https://superuser.com/questions/517986/is-it-possible-to-delete-some-pages-of-a-pdf-document}{command line tools}.
